# Supplementary material for: Simulation and modelling of convective mixing of carbon dioxide in geological formations
Source: arXiv:2501.06090 ancillary file (2025-03-26)
Supplement: Supplementary file 1 [file Supporting_information.pdf]

# Supporting Information for "Simulation and modelling of convective mixing of carbon dioxide in geological formations"

Marco De Paoli[1,2], Francesco Zonta[3], Lea Enzenberger[2], Eliza Coliban[2], and Sergio Pirozzoli[4]

[1]Physics of Fluids Group and Max Planck Center for Complex Fluid Dynamics and J. M. Burgers Centre for Fluid Dynamics, University of Twente, P.O. Box 217, 7500AE Enschede, The Netherlands

[2]Institute of Fluid Mechanics and Heat Transfer, TU Wien, 1060 Vienna, Austria

[3]School of Engineering, Newcastle University, Newcastle upon Tyne NE1 7RU, United Kingdom

[4]Dipartimento di Ingegneria Meccanica e Aerospaziale, Sapienza Università di Roma, 00184 Rome, Italy

## Contents of this file

1. **Text S1** and **Table S1**: Numerical details and simulations details.
2. **Text S2** and **Figure S1**: Grid independence tests.
3. **Text S3** and **Figures S2, S3**: Boundary effects/modes restrictions
4. **Figures S4** to **S6**
5. **Tables S2** to **S3**

## Additional Supporting Information

1. Captions for **Data Set S1**
2. Caption for **Movie S1**
3. Caption for **Movie S2**

## Introduction

This Supporting Information (SI) contains sections providing additional numerical details. In particular, in **Text S1** information about the numerical details is reported and **Table S1** contains the numerical parameters employed for each simulation. Grid independence is discussed in **Text S2** and **Figure S1**. The effect of the boundaries (domain size) on the flux of solute are presented in **Text S3** and **Figures S2-S3**. In addition, **Figures S4** and **S5** are used to provide additional details on the flow dynamics and to validate the model proposed, respectively. A summary of the measurements obtained from the simulations and used to model the flow are provided in **Tables S2-S3**. Finally, the database containing the data obtained (**Data Set S1**) is presented, and a description for the supplementary movies (**Movies S1-S2**) is also provided.

## Text S1. Numerical details

The numerical simulations rely on a solver extensively used for Direct Numerical Simulations (DNS) of wall-bounded neutrally-buoyant and unstably-stratified turbulent flows (Pirozzoli, 2014; Pirozzoli et al., 2017). More recently, it has been employed to resolved Darcy flows in Rayleigh-Bénard configuration (Pirozzoli et al., 2021; De Paoli et al., 2022). The code, written in the Fortran 90 programming language, was run on LUMI-C (LUMI consortium, Finland) using up to 16,384 cores. All simulations were performed for a total time of $t = 100$ (convective units), but simulations at $Ra \geq 2 \times 10^4$, which were run for shorter time (still long enough to capture the entire flow dynamics) due to the large computational cost (see Figure 2). For the largest simulations, we used up to $34 \times 10^9$ grid points corresponding to 4.2 TB/snapshot. We briefly summarize here the numerical scheme, and we refer to Pirozzoli et al. (2021) and De Paoli et al. (2022) for further details.

The numerical simulations rely on the modified version of a second-order finite-difference incompressible flow solver, based on staggered arrangement of the flow variables (Orlandi, 2000). Eq. (7) is advanced in time by means of a hybrid third-order low-storage Runge-Kutta algorithm, whereby the convective terms are handled explicitly and the diffusive terms are handled implicitly, limited to the vertical direction. A special strategy is used here for the solution of the forced Darcy system (6). By disregarding pressure, at each Runge-Kutta sub-step a provisional velocity field is first determined and is then projected to the space of divergence-free vector functions through a correction step. An efficient direct algorithm, based on Fourier expansions along the periodic directions (Kim & Moin, 1985; Orlandi, 2000), is used here for solving the resulting Poisson equation.

The walls are impermeable to the fluid ($\mathbf{u}^* \cdot \mathbf{n} = 0$, with $\mathbf{n}$ the unit vector perpendicular to the boundary), and slip at the top and bottom boundaries is possible. At the upper boundary the concentration is constant and maximum, namely $C^*(y^* = H^*) = C^*_{\text{max}}$, while at the lower boundary a no-flux condition, $\partial C^*(y^* = 0)/\partial y^* = 0$ (i.e. boundary impermeable to the solute) is applied. Periodicity is considered in the wall-parallel directions. The fluid is initially considered still ($\mathbf{u}^* = 0$) and depleted of solute (i.e. saturated with water only, $C^* = 0$). This configuration is representative of an initial step-like concentration profile.

**Table S1.** Summary of the simulations performed in this study. We report the Rayleigh number $Ra$, grid resolution $N_x \times N_y \times N_z$, and domain width in convective ($L$) and diffusive ($\widehat{L} = L\,Ra$) units. Note that $L = L_x^*/H^*$ and $L = L_x^*/H^* = L_z^*/H^*$ in 2D and 3D, respectively.

| Case | Dim. | $Ra$ | $N_x \times N_y \times N_z$ | $L$ | $\widehat{L}$ |
|---|---|---|---|---|---|
| A1 | 2D | $1 \times 10^2$ | $256 \times 16 \times 1$ | 25 | $2.5 \times 10^3$ |
| A2 | 2D | $2 \times 10^2$ | $512 \times 24 \times 1$ | 25 | $5 \times 10^3$ |
| A3 | 2D | $5 \times 10^2$ | $1280 \times 32 \times 1$ | 25 | $1.25 \times 10^4$ |
| A4 | 2D | $1 \times 10^3$ | $2560 \times 48 \times 1$ | 25 | $2.5 \times 10^4$ |
| A5 | 2D | $2 \times 10^3$ | $5120 \times 64 \times 1$ | 25 | $5 \times 10^4$ |
| A6 | 2D | $5 \times 10^3$ | $5120 \times 128 \times 1$ | 10 | $5 \times 10^4$ |
| A7 | 2D | $1 \times 10^4$ | $5120 \times 256 \times 1$ | 5 | $5 \times 10^4$ |
| A8 | 2D | $2 \times 10^4$ | $5120 \times 512 \times 1$ | 2.5 | $5 \times 10^4$ |
| A9 | 2D | $4 \times 10^4$ | $5120 \times 1024 \times 1$ | 1.25 | $5 \times 10^4$ |
| A10 | 2D | $8 \times 10^4$ | $5120 \times 2048 \times 1$ | 0.625 | $5 \times 10^4$ |
| B1 | 3D | $1 \times 10^2$ | $64 \times 16 \times 64$ | 5 | $5 \times 10^2$ |
| B2 | 3D | $2 \times 10^2$ | $128 \times 24 \times 128$ | 5 | $1 \times 10^3$ |
| B3 | 3D | $5 \times 10^2$ | $256 \times 32 \times 256$ | 5 | $2.5 \times 10^3$ |
| B4 | 3D | $1 \times 10^3$ | $512 \times 48 \times 512$ | 5 | $5 \times 10^3$ |
| B5 | 3D | $2 \times 10^3$ | $1024 \times 64 \times 1024$ | 5 | $1 \times 10^4$ |
| B6 | 3D | $5 \times 10^3$ | $1024 \times 128 \times 1024$ | 2 | $1 \times 10^4$ |
| B7 | 3D | $1 \times 10^4$ | $1024 \times 256 \times 1024$ | 1 | $1 \times 10^4$ |
| B8 | 3D | $2 \times 10^4$ | $1024 \times 512 \times 1024$ | 0.5 | $1 \times 10^4$ |
| B9 | 3D | $4 \times 10^4$ | $2048 \times 1024 \times 2048$ | 0.5 | $2 \times 10^4$ |
| B10 | 3D | $8 \times 10^4$ | $4096 \times 2048 \times 4096$ | 0.5 | $4 \times 10^4$ |

The grid resolution in the horizontal directions is uniform and set according to preliminary grid-independence tests. In particular, a cell size of $\Delta\widehat{x} = \Delta\widehat{z} = 9.766$ is appropriate (further details are provided in Text S2). In the vertical direction, an error function stretching was used to cluster more grid points towards the upper (and lower) boundary layer and thus properly capture the processes that take place there. The resolutions and domain widths considered are indicated in Tab. S1. Given the slightly sub-linear growth of the concentration gradients (Zhu et al., 2024), the number of points in each direction was increased proportionally to $Ra$. Time stepping is chosen to guarantee a Courant-Friedrichs-Lewy (CFL) number about unity for all

the simulations. Special time step restrictions were implemented for some flow regimes: to fully capture the dynamics during the diffusive regime, the time step is set to $\Delta\widehat{t} = 1$; during the shut-down phase, the velocities are very low and an upper limit for the time-steps is chosen regardless of the CFL-condition. To numerically implement the initial condition discussed in Sec. 2.1, we consider that such a step-like concentration profile allows to determine an analytical self-similar solution of Eq. (7) for the evolution of the concentration field (Slim, 2014; De Paoli et al., 2017):

$$C(x, y, t) = 1 + \text{erf}\left[\frac{(y-1)\,Ra}{\sqrt{4t\,Ra}}\right]. \tag{S1}$$

In order to achieve the same initial condition for all the simulations performed, we initialize the concentration field as in Eq. (S1) with an initial time $t_0 = 250/\,Ra$, which is the first instant considered. Finally, a random perturbation $a$ (white noise) modulated by a coefficient (amplitude) $\epsilon = 0.01$ is added such that the field at the first instant is defined as:

$$C(x, y, z, t_0) = 1 + \text{erf}\left[\frac{(y-1)\,Ra}{\sqrt{4t_0\,Ra}}\right][1 + \epsilon(a - 0.5)]. \tag{S2}$$

The amplitude of the initial perturbation employed to trigger the flow, $\epsilon$, controls the time at which the onset of convection occurs, i.e., it controls the time at which fingers form (Slim & Ramakrishnan, 2010). In quantitative terms, this time has been defined as the instant corresponding to the initial growth of the finger-tip velocity (Elenius & Johannsen, 2012) or of the perturbation amplitude (Slim, 2014), among other definitions (Riaz et al., 2006). Amplitude and wavelength of the perturbation have an effect on the transient part preceding the constant flux regime, in particular on the minimum and maximum values of the flux, and on the times at which these values are achieved. After a detailed analysis of previous works, Riaz and Cinar (2014) concluded that the onset time for convection depends mainly on the amplitude of the initial perturbation, and that it decreases with an increase of the amplitude. Concerning the perturbation structure,

it was observed, for example, that shorter wavelength perturbations start growing earlier than small wavenumber perturbations, generating less intense convection and ultimately leading to a lower value of the maximum flux (Slim, 2014). The initial condition is completely absorbed after the constant flux regime: for sufficiently large $Ra$ (simulations A6-A10 and B6-10 in Tab. S1) the behavior of the system is independent of the initial perturbation (Slim, 2014), and therefore the flow can be considered independent of the initial condition.

## Text S2. Grid independence tests

To investigate the influence of the resolution, a grid sensitivity study has been performed. We considered a squared (cubic) domain, in 2D (3D) at the Rayleigh number $Ra = 10^4$. The grid is uniform in horizontal direction, while in vertical direction points are clustered towards the upper and lower horizontal walls, where small-scale structures and large concentration gradients are

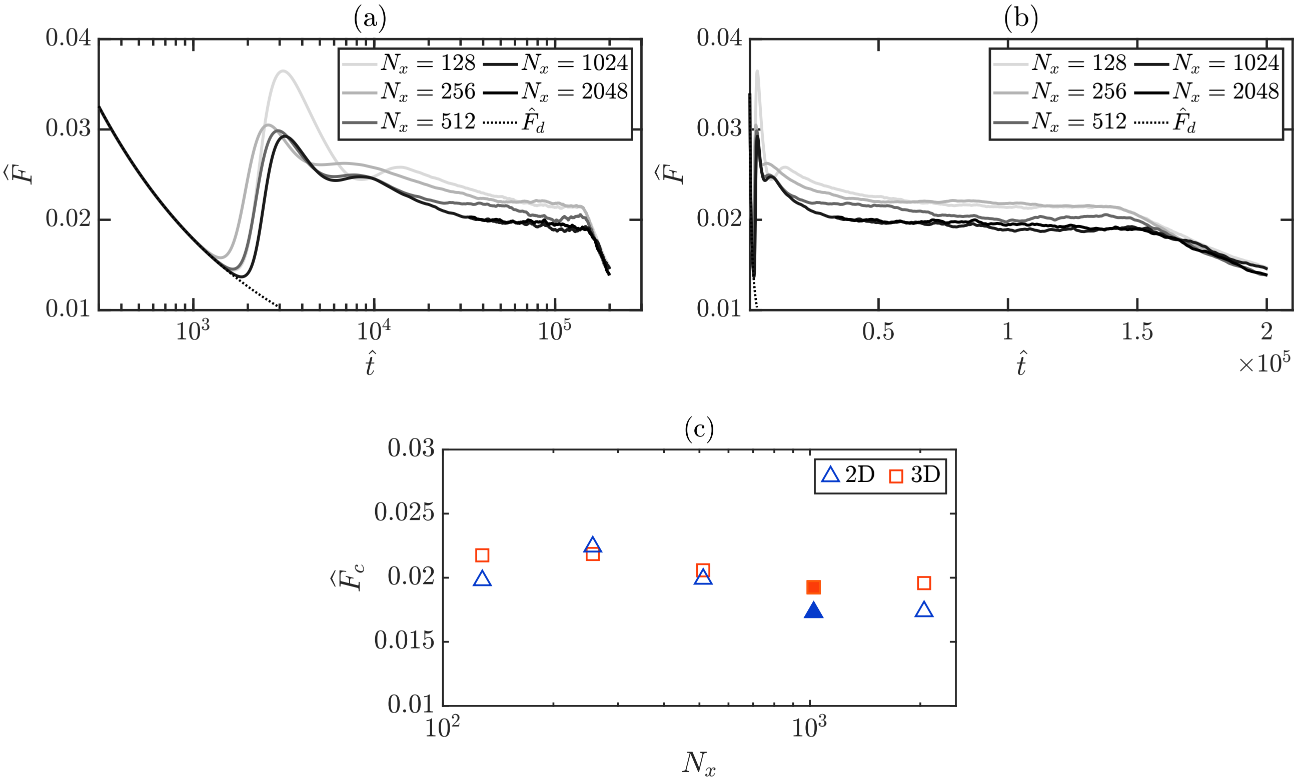


**Figure S1.** Grid sensitivity for the simulation at $Ra = 10^4$. (a-b) Time-dependent behavior of the dissolution fluxes $\widehat{F}$ for the 3D simulations (a - time in logarithmic scale, b - time in linear scale). The number of points used in horizontal direction ($N_x = N_z$) is indicated, as well as the initial diffusive flux ($\widehat{F}_d$, dotted line). (c) Time-averaged dissolution rate $\widehat{F}_c$ obtained during the constant flux regime (defined as in the main text), for both 2D (blue triangles) and 3D (red squares) simulations and as a function of the number of nodes. Filled symbols indicated the value employed in the production simulations.

present. The points distribution in the wall-normal direction is obtained using an error function. First we fixed the number of grid points in vertical direction and we investigated the effect of the horizontal resolution, and then we repeated the process for the vertical direction.

In Figs. S1(a,b), we analyzed the instantaneous dissolution flux at the top boundary with $N_y = 256$ and variable $N_x = N_z$. We observe no significant variation for $N_x \geq 1024$. The same trend is observed in the flux averaged during the constant flux regime, $\widehat{F}_c$, reported in Fig. S1(c) and defined in the main text. In the 2D case, the flux matches the results obtained in previous studies, namely $\widehat{F}_c = 0.017$ (Pau et al., 2010; Slim, 2014; De Paoli et al., 2017; Wen et al., 2018). As a result, the grid resolution in horizontal direction is set to $N_x(= N_z) = 1024$ for $L = 1$ in both 2D and 3D simulations.

The influence of the number of grid points in vertical direction, $N_y$, has also been considered and the same procedure applied in horizontal direction has been repeated, with $N_x$ (and $N_z$) fixed and equal to 1024. The analysis of the flux (not reported) indicates that $N_y = 256$ is sufficient. We conclude that a grid size $N_x \times N_y(\times N_z) = 1024 \times 256(\times 1024)$ is appropriate for $Ra = 1 \times 10^4$ with $L = 1$, corresponding to a horizontal cell size $\Delta\widehat{x} = L\,Ra\,/N_x = 9.766$ (in diffusive units), in agreement with previous works (Slim, 2014; Pirozzoli et al., 2021). The number of grid points is set proportionally to $Ra$ and $L$ for all the simulations considered, thus ensuring the same cell size in diffusive units.

**Text S3. Boundary effects/modes restrictions**

To account for the effects of the periodic boundary conditions and to assess the requirements in terms of domain size, we performed additional simulations in which the horizontal domain width is varied, corresponding to a variation of $L$. The goal is to identify a domain width that

is sufficiently small, to keep the computational costs accessible, but large enough to capture all the flow features.

The effect of $L$ is quantified again looking at the dissolution rate $\widehat{F}$, which we report in Fig. S2 for 3D simulations at $Ra = 10^4$. We observe that the aspect ratio has a strong influence on the fluctuations of the dissolution flux, whereas the mean value during the constant flux regime remains nearly unaffected (see Fig. S3). We observe that the constant flux $\widehat{F}_c$ is independent of $L$ within the range of values considered, both in 3D and in 2D simulations (Fig. S3a), although a weak increase is observed for $L = 1/2$ in the 2D case. In contrast, the fluctuations of the flux during the constant flux, quantified by the standard deviation $\sigma$, are sensibly affected by the domain size (Fig. S3b). Therefore, we conclude that at $Ra = 10^4$ an aspect ratio $L = 5$ for the 2D case and $L = 1$ for the 3D case is required. The fact that a smaller $L$ is needed for 3D compared to 2D simulations is not surprising: for a fixed $L$, the additional spatial dimension available in 3D implies a larger area of sampling compared to the 2D case.

The domain width at all $Ra$ considered is varied proportionally, and thus such that $\widehat{L} \geq 10^4$. Only for the low-$Ra$ simulations, in which the constant flux regime is not achieved, the domain width is limited to $L = 5$ (3D) and $L = 25$ (2D). The resolution was also adapted such that the cell size is kept constant (in horizontal direction it reads $\Delta\widehat{x} = \Delta\widehat{z} = 9.766$). Not doing so would result in poor resolution at low $Ra$ and unnecessarily fine resolution at high $Ra$.

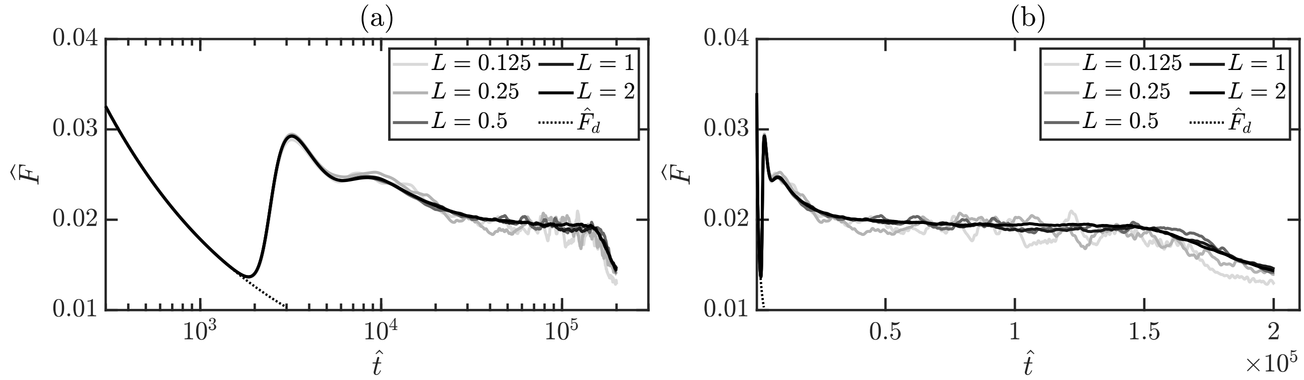


**Figure S2.** Effect of the horizontal domain size, $L$, on the time dependent dissolution rate at the top wall in 3D simulations ($Ra = 10^4$, a - time in logarithmic scale, b - time in linear scale). The initial flux during the diffusive phase ($\widehat{F}_d$, dotted line) is also reported.

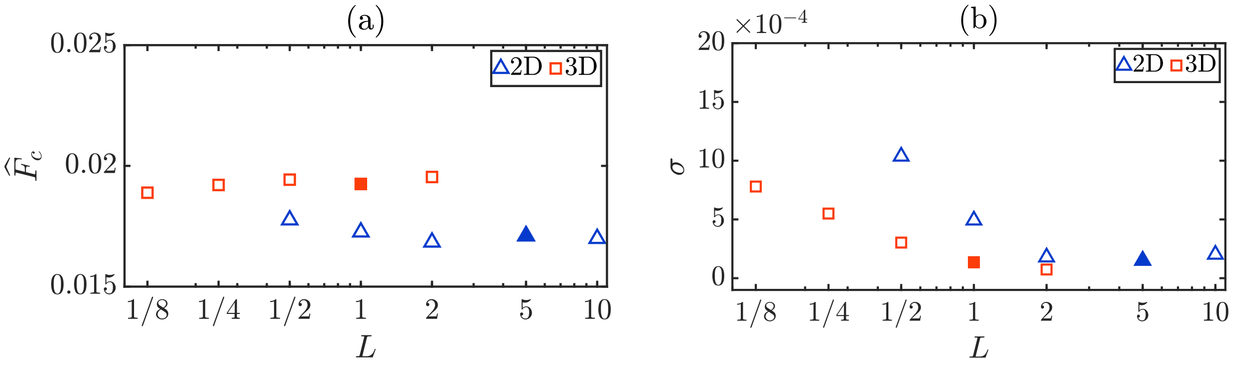


**Figure S3.** Effect of the horizontal domain size ($L$) for both 2D and 3D simulations at $Ra = 10^4$ on (a) the average dissolution flux during the constant flux regime, $\widehat{F}_c$, and (b) the mean standard deviation $\sigma$ of the flux $\widehat{F}$ during the constant flux regime. Filled symbols indicate the value of $L$ employed in 2D (blue) and 3D (red) for the production simulations.

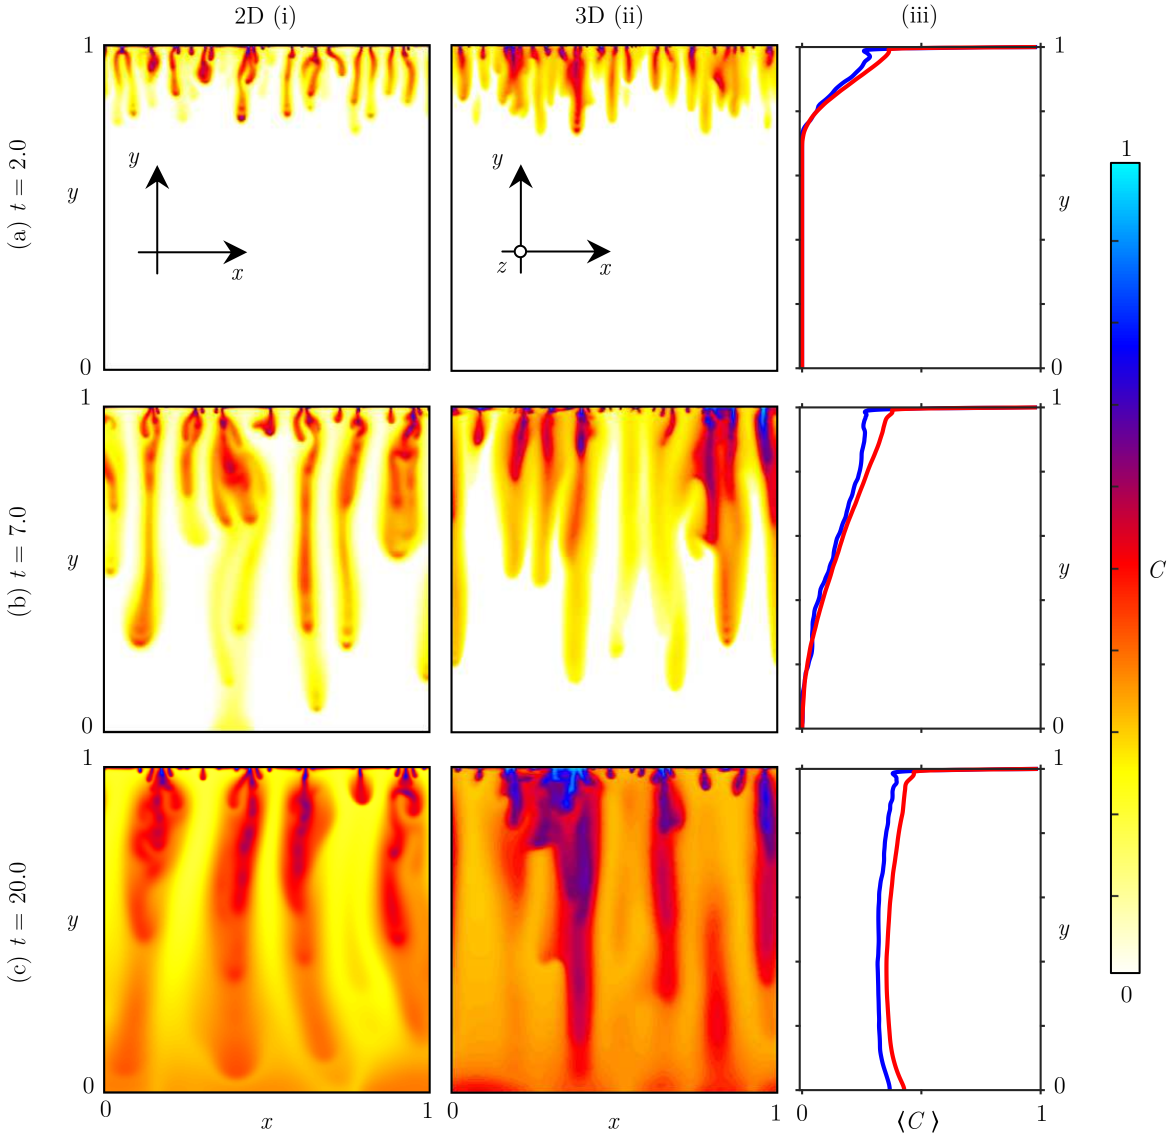


**Figure S4.** Vertical concentration distributions for $Ra = 10^4$ at different time instants, namely $t = 2$ (panels a), 7 (panels b) and 20 (panels c) for the 2D simulations (left column) and 3D simulations (center column), together with the horizontally-averaged concentration $\langle C \rangle$, shown over the height of the computational domain (right column), where the blue lines represent the 2D data (simulation A7) and the red lines the 3D data (simulation B7).

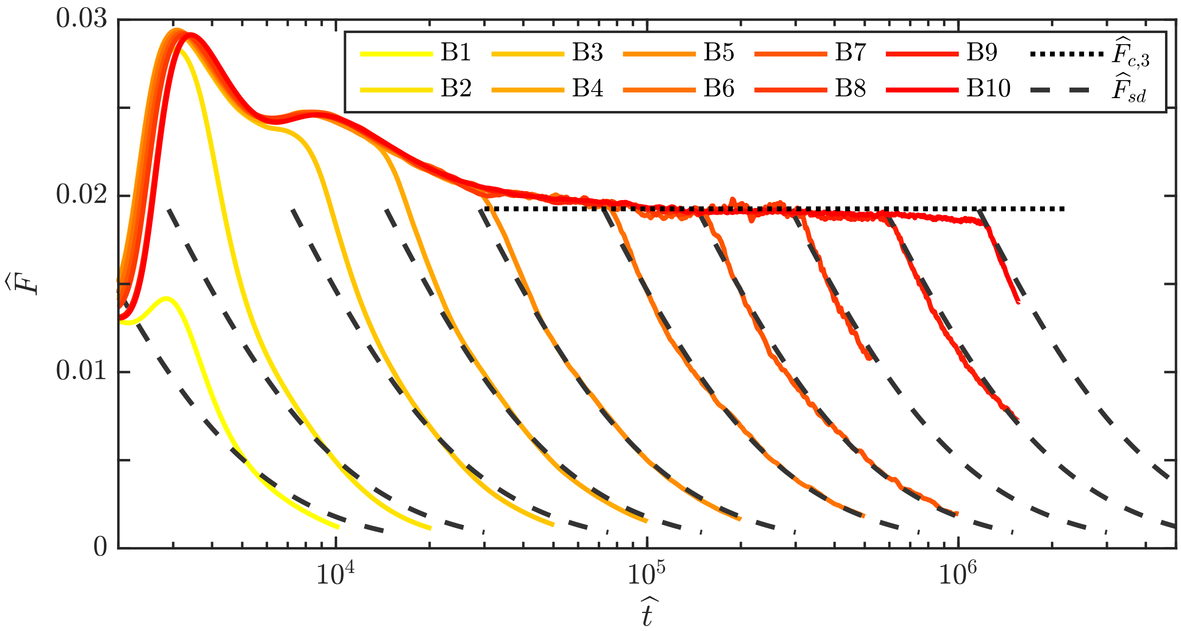


**Figure S5.** Comparison of the box-model prediction during the shutdown phase against the numerical results in the 3D case. Simulations (solid lines) are compared against the model ($\widehat{F}_{sd}$, (16), dashed lines). The details of the models are presented in Sec. 3.1.3.

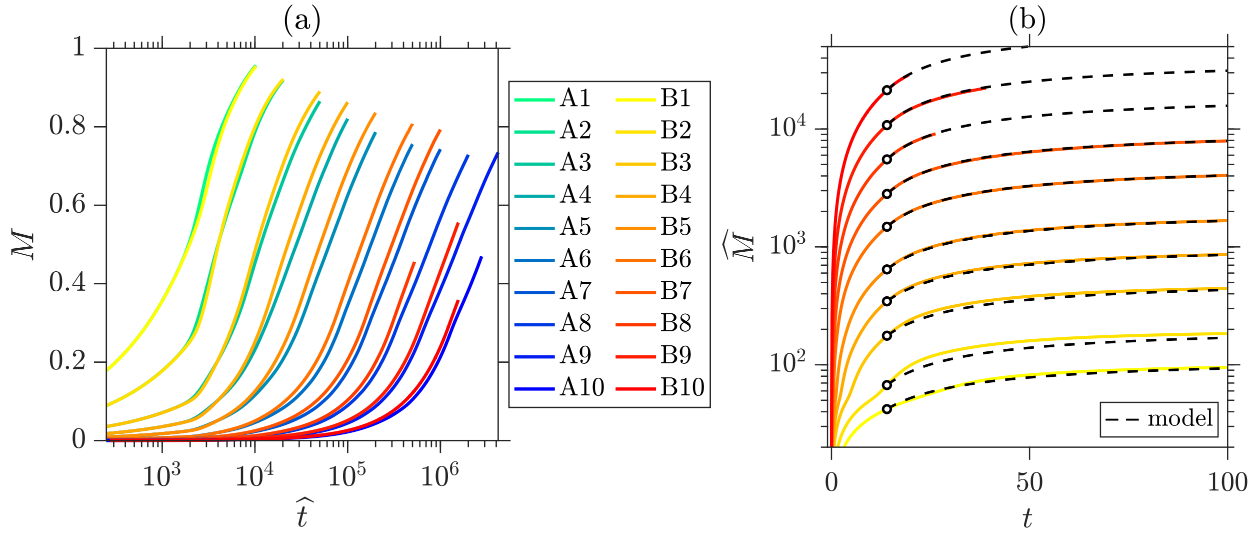


**Figure S6.** Evolution of the volume of solute dissolved and expressed in (a) convective units $M$ and (b) diffusive units $\widehat{M} = M\,Ra$, see Eq. (17). In (a), both 2D and 3D simulations are shown (labeled as A# and B#, respectively). In (b), only 3D numerical results are presented together with the model predictions (Eq. (18), dashed lines). The symbols indicates the first instant at which the model is shown (see Sec. 3.2 for further details).

**Table S2.** Summary of the simulations performed in this study. We report the Rayleigh number $Ra$, the dissolution flux $\widehat{F}$ and the corresponding standard deviation $\sigma(\widehat{F})$ during the constant flux regime, defined here as $2 \times 10^4 \leq \widehat{t} \leq 16\,Ra$ in 2D and $4 \times 10^4 < t < 14\,Ra$ in 3D. Finally, the values of the characteristic length scale obtained from the power-averaged mean wave number ($\widehat{\lambda}_c = 1/\widehat{k}$) are also reported. Further numerical details are provided in Tab. S1.

| Case | Dim. | $Ra$ | $\widehat{F}_c$ | $\sigma(\widehat{F})$ | $\widehat{\lambda}_c$ | $\sigma(\widehat{\lambda})$ |
|---|---|---|---|---|---|---|
| A1 | 2D | $1 \times 10^2$ | - | - | - | - |
| A2 | 2D | $2 \times 10^2$ | - | - | - | - |
| A3 | 2D | $5 \times 10^2$ | - | - | - | - |
| A4 | 2D | $1 \times 10^3$ | - | - | - | - |
| A5 | 2D | $2 \times 10^3$ | - | - | - | - |
| A6 | 2D | $5 \times 10^3$ | 0.01672 | $3.167 \times 10^{-4}$ | 489.3801 | 32.3486 |
| A7 | 2D | $1 \times 10^4$ | 0.01708 | $3.949 \times 10^{-4}$ | 457.5535 | 36.0866 |
| A8 | 2D | $2 \times 10^4$ | 0.01688 | $5.962 \times 10^{-4}$ | 471.6531 | 57.4772 |
| A9 | 2D | $4 \times 10^4$ | 0.01715 | $4.460 \times 10^{-4}$ | 422.7691 | 34.5794 |
| A10 | 2D | $8 \times 10^4$ | 0.01705 | $6.835 \times 10^{-4}$ | 434.3080 | 59.8472 |
| B1 | 3D | $1 \times 10^2$ | - | - | - | - |
| B2 | 3D | $2 \times 10^2$ | - | - | - | - |
| B3 | 3D | $5 \times 10^2$ | - | - | - | - |
| B4 | 3D | $1 \times 10^3$ | - | - | - | - |
| B5 | 3D | $2 \times 10^3$ | - | - | - | - |
| B6 | 3D | $5 \times 10^3$ | 0.01975 | $2.125 \times 10^{-4}$ | 253.7446 | 9.4345 |
| B7 | 3D | $1 \times 10^4$ | 0.01926 | $3.961 \times 10^{-4}$ | 282.6929 | 23.0193 |
| B8 | 3D | $2 \times 10^4$ | 0.01933 | $2.916 \times 10^{-4}$ | 281.7261 | 22.2302 |
| B9 | 3D | $4 \times 10^4$ | 0.01903 | $2.679 \times 10^{-4}$ | 288.7920 | 18.7458 |
| B10 | 3D | $8 \times 10^4$ | 0.01894 | $2.536 \times 10^{-4}$ | 278.4132 | 17.7501 |

**Table S3.** Summary of parameters employed in 2D and 3D cases. "measurements" indicates the time range used to define the constant flux regime, and over which the quantities $\widehat{F}_c$ and $\widehat{\lambda}_c$ are computed; "model" refers to the parameters used in Eqs. (16) and (19).

| | measurements | | | | model | | | |
|---|---|---|---|---|---|---|---|---|
| Dim. | $\widehat{t}_{c,1}$ | $\widehat{t}_{c,2}$ | $\widehat{F}_c$ | $\widehat{\lambda}_c$ | $\widehat{t}_1$ | $\widehat{t}_2 = t_{sd}\,Ra$ | $c_0$ | $Ra_{cr}$ |
| 2D | $2 \times 10^4$ | $16\,Ra$ | 0.016973 | 455 | 4419.7 | $16\,Ra$ | 0.2716 | 31.5 |
| 3D | $4 \times 10^4$ | $14\,Ra$ | 0.019264 | 277 | 3431.0 | $14\,Ra$ | 0.2697 | 27.0 |

**Data Set S1.** A database containing the data of flux for all simulations performed is available (De Paoli et al., 2025). The following quantities are provided:

- Rayleigh-Darcy number: $Ra$, see Eq. (8) ;
- Time in diffusive units: $\widehat{t}$, see Eq. (9) ;
- Simulation time step in diffusive units: $\Delta\widehat{t}$ ;
- Flux at the top boundary: $\widehat{F}(\widehat{t})$, see Eq. (10) ;
- Volume of solute dissolved $\widehat{M}(\widehat{t})$, see Eq. (17) ;

**Movie S1.** Evolution of simulation A7 ($Ra = 10^4$, only a small portion of the domain in horizontal direction is considered). Top left panel: concentration field. Bottom left panel: Close-up view of the top boundary layer. The process of fingers formation and merging is visible. Center panel: space-time map, $C(x, y = 0.995, t)$, relative to the concentration distribution close to the upper boundary (the height at which the concentration is taken, $y = 0.995$, is indicated by the arrow in the top left panel). The dark blue branches appearing during the constant flux regime ($t < 16$) correspond to the presence of plumes that are persistent in time and space (see Sec. 3.1.2). The beginning of the shutdown phase ($t \approx 16$) is marked by the saturation of the upper boundary layer (blue region in the space time map), and in this regime the plumes are even more persistent. Right panel: Evolution of the dissolution rate at the upper boundary, $\widehat{F}$, as a function of time.

**Movie S2.** Evolution of the near-wall flow structures for the $Ra = 10^4$ (simulations B7 in Tab. S1). The concentration distribution over a horizontal slice taken at $y = 0.995$ is reported. The convective time, $0 \leq t \leq 85$, indicated in the top left corner, spans over all the regimes. At

this wall-normal location and $Ra$, fingers appear at $t \approx 1$. They subsequently merge into larger and statistically-steady cells ($4 \leq t \leq 14$). Finally, the driving reduces as a result of the domain saturation, and the near-wall cells dynamics slows progressively down.

## References


De Paoli, M., Pirozzoli, S., Zonta, F., & Soldati, A. (2022). Strong Rayleigh–Darcy convection regime in three-dimensional porous media. *J. Fluid Mech.*, *943*, A51. Retrieved from https://doi.org/10.1017/jfm.2022.461 doi: 10.1017/jfm.2022.461

De Paoli, M., Zonta, F., Enzenberger, L., Coliban, E., & Pirozzoli, S. (2025, 01). Simulation and modelling of convective mixing of carbon dioxide in geological formations.. Retrieved from https://doi.org/10.6084/m9.figshare.28175018 doi: 10.6084/m9.figshare.28175018

De Paoli, M., Zonta, F., & Soldati, A. (2017). Dissolution in anisotropic porous media: Modelling convection regimes from onset to shutdown. *Phys. Fluids (1994-present)*, *29*(2), 026601.

Elenius, M., & Johannsen, K. (2012). On the time scales of nonlinear instability in miscible displacement porous media flow. *Comput. Geosci.*, *16*(4), 901–911.

Kim, J., & Moin, P. (1985). Application of a fractional-step method to incompressible Navier-Stokes equations. *J. Comput. Phys.*, *59*, 308–323.

Orlandi, P. (2000). *Fluid flow phenomena: a numerical toolkit.* Kluwer.

Pau, G. S., Bell, J. B., Pruess, K., Almgren, A. S., Lijewski, M. J., & Zhang, K. (2010). High-resolution simulation and characterization of density-driven flow in CO2 storage in saline aquifers. *Adv. Water Resour.*, *33*(4), 443–455. Retrieved from https://www.sciencedirect.com/science/article/pii/S0309170810000217 doi: https://doi.org/10.1016/j.advwatres.2010.01.009

Pirozzoli, S. (2014). Revisiting the mixing-length hypothesis in the outer part of turbulent wall layers: mean flow and wall friction. *J. Fluid Mech.*, *745*, 378–397.

Pirozzoli, S., Bernardini, M., Verzicco, R., & Orlandi, P. (2017). Mixed convection in turbulent channels with unstable stratification. *J. Fluid Mech.*, *821*, 482–516.

Pirozzoli, S., De Paoli, M., Zonta, F., & Soldati, A. (2021). Towards the ultimate regime in Rayleigh–Darcy convection. *J. Fluid Mech.*, *911*, R4.

Riaz, A., & Cinar, Y. (2014). Carbon dioxide sequestration in saline formations: Part I–Review of the modeling of solubility trapping. *J. Petrol. Sci. Eng.*, *124*, 367–380.

Riaz, A., Hesse, M., Tchelepi, H., & Orr, F. (2006). Onset of convection in a gravitationally unstable diffusive boundary layer in porous media. *J. Fluid Mech.*, *548*, 87–111.

Slim, A. (2014). Solutal-convection regimes in a two-dimensional porous medium. *J. Fluid Mech.*, *741*, 461–491.

Slim, A., & Ramakrishnan, T. (2010). Onset and cessation of time-dependent, dissolution-driven convection in porous media. *Phys. Fluids (1994-present)*, *22*(12), 124103.

Wen, B., Akhbari, D., Zhang, L., & Hesse, M. (2018). Convective carbon dioxide dissolution in a closed porous medium at low pressure. *J. Fluid Mech*, *854*, 56-87.

Zhu, X., Fu, Y., & De Paoli, M. (2024). Transport scaling in porous media convection. *J. Fluid Mech.*, *991*, A4.
